# Supplementary material for: SCOL: Supervised Contrastive Ordinal Loss for Abdominal Aortic Calcification Scoring on Vertebral Fracture Assessment Scans
Source: arXiv:2307.12006 source file (2023-07-22)
Supplement: Supplementary file 1 [file Paper1923Supplementary.pdf]

# SCOL: Supervised Contrastive Ordinal Loss for Abdominal Aortic Calcification Scoring on Vertebral Fracture Assessment Scans

## Supplementary Material

Afsah Saleem et al.

afsah.saleem@ecu.edu.au

**Example of AAC Scoring:** If  $l$  is the length of calcification in the abdominal aorta (red line in Fig. 1(a)) and  $h$  is the height of any one vertebral body from L1 to L4, then the AAC-24 score for the given example is calculated as:

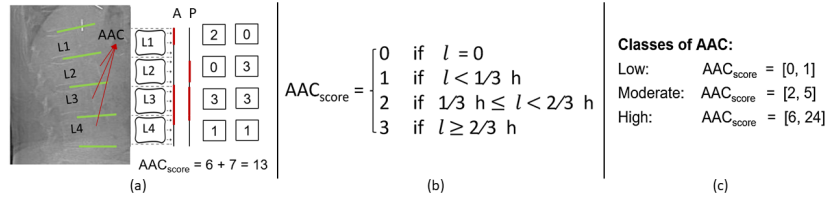

**Fig. 1.** Example of AAC scoring. In (a) A: Anterior wall, P: Posterior wall.

**T-SNE plot to visualize interclass-separation and the intra-class variations:** It can be easily seen in Fig. 2(a) that the distribution of feature embeddings produced by RMSE loss is mitigated and overlap with each other. It means RMSE loss that AAC scores are not completely separable. In comparison, it can be seen in Fig. 2 (b) that our proposed loss SCOL suppresses the intra-class variations, enhances the inter-class similarities, and generate a separable distribution of feature embeddings in latent space.

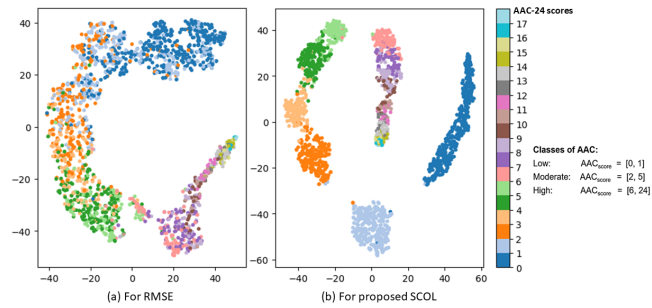

**Fig. 2.** T-SNE visualization: (a) Baseline trained with RMSE, (b) Proposed DCOL trained with SCOL. RMSE: Root Mean Squared Error, DCOL: Dual-encoder Contrastive Ordinal Learning, SCOL: Supervised Contrastive Ordinal Loss

**Training Strategy:** For each fold, we divide the dataset into train test split using 10-fold cross-validation in a stratified manner. In each fold, 90% of data was used for training and tested on the remaining 10% of data. There was no overlap between train, and test splits in any fold. Thus, we train 10 distinct networks for the 10 different folds. Each network is trained on 1,722 scans which comprise of 1550 training scans and 172 scans in the validation set. The network is then tested on 192 unseen test images. In this way, all 10 networks are trained on a distinct training/ validation set and tested on an unseen dataset of 192 images each. For a fair comparison, we have used the same cross-validation strategy as the SOTA [7,18]. To avoid over-fitting, LR is decreased on the plateau with the factor of 0.2, and early stopping is performed with the tolerance of 5 epochs, while optimizing the loss.

**Confusion matrices for Table 1, Table 2, Table 3:**

| Actual Values | Predicted Values |           |      |     |
|---------------|------------------|-----------|------|-----|
|               | Low              | Mod erate | High |     |
|               | Low              | 512       | 251  | 1   |
|               | Mod erate        | 208       | 501  | 5   |
|               | High             | 0         | 54   | 382 |

Baseline

| Actual Values | Predicted Values |           |      |     |
|---------------|------------------|-----------|------|-----|
|               | Low              | Mod erate | High |     |
|               | Low              | 578       | 186  | 0   |
|               | Mod erate        | 210       | 495  | 9   |
|               | High             | 0         | 58   | 378 |

(b) SupCon

| Actual Values | Predicted Values |           |      |     |
|---------------|------------------|-----------|------|-----|
|               | Low              | Mod erate | High |     |
|               | Low              | 547       | 217  | 0   |
|               | Mod erate        | 184       | 524  | 6   |
|               | High             | 0         | 53   | 383 |

(c) AdaCon

| Actual Values | Predicted Values |           |      |     |
|---------------|------------------|-----------|------|-----|
|               | Low              | Mod erate | High |     |
|               | Low              | 574       | 190  | 0   |
|               | Mod erate        | 182       | 527  | 5   |
|               | High             | 0         | 46   | 390 |

Proposed Method

**Fig. 3.** Confusion matrices for Table 1. (a) Baseline trained with RMSE& (b) SupCon, (c) AdaCon (d) Proposed SCOL. SupCon, AdaCon, and SCOL are trained with the proposed Dual-encoder framework.

| Actual Values | Predicted Values |           |      |     |
|---------------|------------------|-----------|------|-----|
|               | Low              | Mod erate | High |     |
|               | Low              | 512       | 251  | 1   |
|               | Mod erate        | 208       | 501  | 5   |
|               | High             | 0         | 54   | 382 |

(a) Baseline

| Actual Values | Predicted Values |           |      |     |
|---------------|------------------|-----------|------|-----|
|               | Low              | Mod erate | High |     |
|               | Low              | 574       | 190  | 0   |
|               | Mod erate        | 182       | 527  | 5   |
|               | High             | 0         | 46   | 390 |

(b) Proposed Method

| Actual Values | Predicted Values |           |      |     |
|---------------|------------------|-----------|------|-----|
|               | Low              | Mod erate | High |     |
|               | Low              | 680       | 139  | 10  |
|               | Mod erate        | 121       | 266  | 58  |
|               | High             | 9         | 111  | 522 |

(c) Baseline

| Actual Values | Predicted Values |           |      |     |
|---------------|------------------|-----------|------|-----|
|               | Low              | Mod erate | High |     |
|               | Low              | 714       | 104  | 11  |
|               | Mod erate        | 113       | 280  | 52  |
|               | High             | 6         | 104  | 532 |

(d) Proposed Method

**Fig. 4.** Confusion matrices for Table 1. (a) & (b) for Hologic dataset, (c) & (d) for iDXA GE dataset.

| Actual Values | Predicted Values |           |      |     |
|---------------|------------------|-----------|------|-----|
|               | Low              | Mod erate | High |     |
|               | Low              | 460       | 308  | 61  |
|               | Mod erate        | 132       | 264  | 49  |
|               | High             | 52        | 238  | 352 |

(a) Reid et al.

| Actual Values | Predicted Values |           |      |     |
|---------------|------------------|-----------|------|-----|
|               | Low              | Mod erate | High |     |
|               | Low              | 716       | 85   | 28  |
|               | Mod erate        | 201       | 167  | 77  |
|               | High             | 21        | 106  | 515 |

(b) Gilani et al.

| Actual Values | Predicted Values |           |      |     |
|---------------|------------------|-----------|------|-----|
|               | Low              | Mod erate | High |     |
|               | Low              | 714       | 104  | 11  |
|               | Mod erate        | 113       | 280  | 52  |
|               | High             | 6         | 104  | 532 |

(c) Proposed DOCL

**Fig. 5.** Confusion matrices for Table 3.
